# Supplementary material for: The effect of tides on the Sculptor dwarf spheroidal galaxy
Source: arXiv:1904.10461 source file (2019-06-28)
Supplement: Supplementary file 1 [file EM18.tex]

\Section{An extreme orbital case} \label{app:em18}
